# Supplementary material for: Understanding and reducing errors in density functional calculations
Source: arXiv:1212.3054 source file (2013-07-29)
Supplement: Supplementary file 1 [file KSB13-2-SI.pdf]

## Understanding and reducing errors in density functional calculations

Min-Cheol Kim,<sup>1</sup> Eunji Sim\*,<sup>1</sup> and Kieron Burke<sup>2</sup>

<sup>1</sup>*Department of Chemistry and Institute of Nano-Bio Molecular Assemblies,  
Yonsei University, 50 Yonsei-ro Seodaemun-gu, Seoul 120-749 Korea*

<sup>2</sup>*Department of Chemistry, University of California, Irvine, CA, 92697,  
USA*

(Dated: 10 June 2013)

## I. TWO ELECTRON SYSTEMS

To make Fig. 1, we carefully interpolated accurate QMC energies<sup>1,2</sup> from  $Z^{-1} = 1$  to 0, and repeated this procedure applying PBE to the exact densities to find  $\Delta E_F(Z)$ . We also used Turbomole<sup>3</sup> to solve for self-consistent PBE energies and the eigenvalue. For  $Z \leq Z_c$ , the eigenvalue is pinned to 0, and an increasing fraction of an electron escapes. To achieve self consistency, we decreased the occupation of the orbital from 2 until we find an occupation at which the total energy converges and the eigenvalue vanishes.

## II. HO·H<sub>2</sub>O COMPLEX

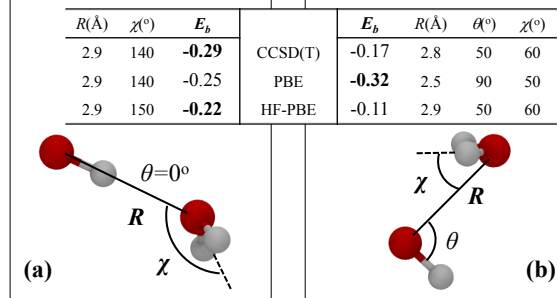

FIG. S1. Binding energies in eV of HO·H<sub>2</sub>O calculated with various methods for (a) hydrogen-bonding structure and (b) hemi-bonding structure.

PES scan results for HO·H<sub>2</sub>O complex are shown in Fig. S1. Self-consistent PBE greatly overstabilizes the hemi bond, resulting in a strong, unphysical hemi-bonding minimum,  $\Delta\epsilon_g^{\text{PBE}}$  is less than 1 eV. CCSD(T) and HF-PBE, on the other hand, give the hydrogen-bonding geometry as the global minimum.

### III. $\text{H}_2^+$ DISSOCIATION

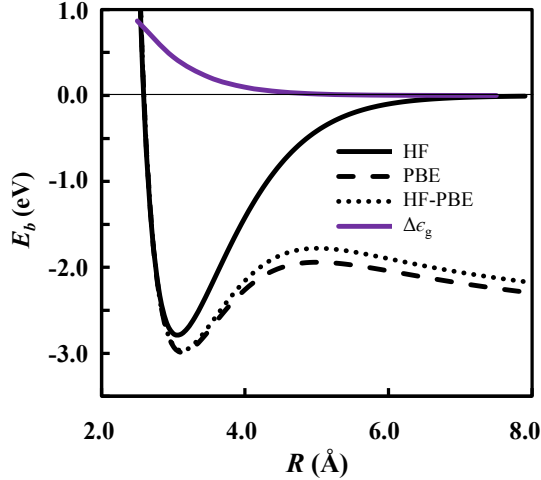

FIG. S2. Binding energy of  $\text{H}_2^+$  as a function of separation in several calculations, and the PBE HOMO-LUMO gap.

Dissociation of  $\text{H}_2^+$  with a standard functional is shown in Fig. S2. We compare self-consistent calculations with the HF-DFT method and HF method. The HOMO-LUMO gap ( $\Delta\epsilon_g$ ) is also shown in the figure.

### IV. CALCULATION DETAILS

Self-consistent PBE calculation for two electron systems were performed with an aug-cc-pV6Z basis set<sup>5</sup>. For all other calculations (e.g. NaCl dissociation, OH radical complexes,  $\text{H}_2^+$  dissociation), self-consistent PBE and HF-PBE calculations were performed with an aug-cc-pVTZ<sup>6-8</sup> basis. All calculations mentioned above were performed with the Turbomole<sup>3</sup> program. SCF convergence and density convergence criteria of  $10^{-8}$  were used, and grid size of 6 were used for PBE calculations.

### REFERENCES

- <sup>1</sup>C. J. Umrigar and X. Gonze, “Accurate exchange-correlation potentials and total-energy components for the helium isoelectronic series,” Phys. Rev. A, **50**, 3827 (1994).

- <sup>2</sup>C.-J. Huang and C. J. Umrigar, “Local correlation energies of two-electron atoms and model systems,” *Phys. Rev. A*, **56**, 290 (1997).
- <sup>3</sup>“TURBOMOLE V6.2, TURBOMOLE GmbH, Karlsruhe, Germany, 2010, <http://www.turbomole.com>.”.
- <sup>4</sup>D. M. Chipman, “Hemibonding between hydroxyl radical and water,” *J. Phys. Chem. A*, **115**, 1161 (2011).
- <sup>5</sup>T. Van Mourik, A. K. Wilson, and T. H. Dunning, “Benchmark calculations with correlated molecular wavefunctions. xiii. potential energy curves for he2, ne2 and ar2 using correlation consistent basis sets through augmented sextuple zeta,” *Mol. Phys.*, **96**, 529 (1999).
- <sup>6</sup>R. A. Kendall, J. Thom H. Dunning, and R. J. Harrison, “Electron affinities of the first-row atoms revisited. systematic basis sets and wave functions,” *J. Chem. Phys.*, **96**, 6796 (1992).
- <sup>7</sup>D. E. Woon and J. Thom H. Dunning, “Gaussian basis sets for use in correlated molecular calculations. iii. the atoms aluminum through argon,” *J. Chem. Phys.*, **98**, 1358 (1993).
- <sup>8</sup>B. Prascher, D. Woon, K. Peterson, J. Dunning, ThomH., and A. Wilson, “Gaussian basis sets for use in correlated molecular calculations. vii. valence, core-valence, and scalar relativistic basis sets for li, be, na, and mg,” *Theoret. Chem. Acc.*, **128**, 69 (2011).
